# Supplementary material for: Multimodal Speech Emotion Recognition Using Audio and Text
Source: arXiv:1810.04635 source file (2018-10-10)
Supplement: Supplementary file 1 [file fig_confusion_appendix.tex]

\begin{figure*}[htbp!]
% \small
\centering
\bigskip
\subfigure[ARE]{\label{fig_confusion_ARE_appendix}\includegraphics[width=0.45\columnwidth]{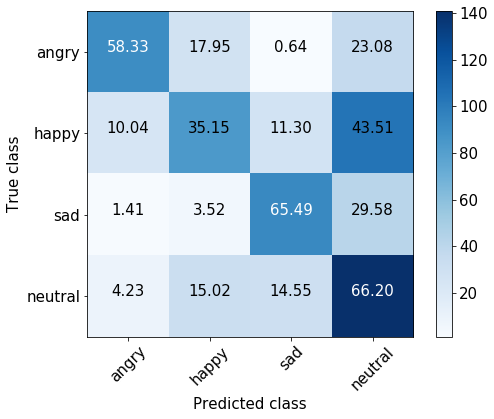}}
\qquad
\subfigure[TRE]{\label{fig_confusion_TRE_appendix}\includegraphics[width=0.45\columnwidth]{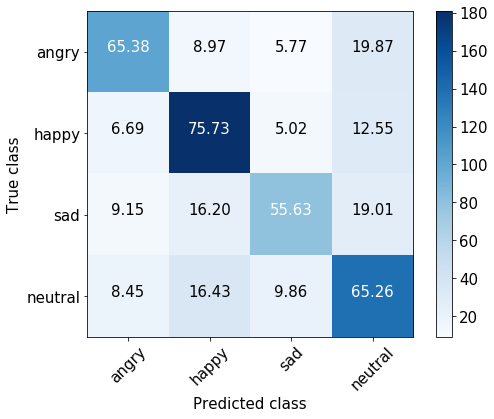}}

\bigskip

\subfigure[MDRE]
{\label{fig_confusion_MDRE_appendix}\includegraphics[width=0.45\columnwidth]{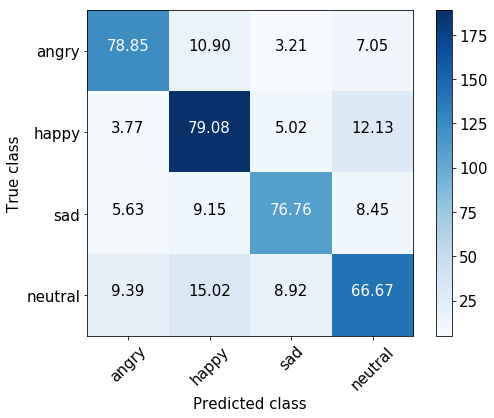}}
\qquad
\subfigure[MDREA]{\label{fig_confusion_MDREA_appendix}\includegraphics[width=0.45\columnwidth]{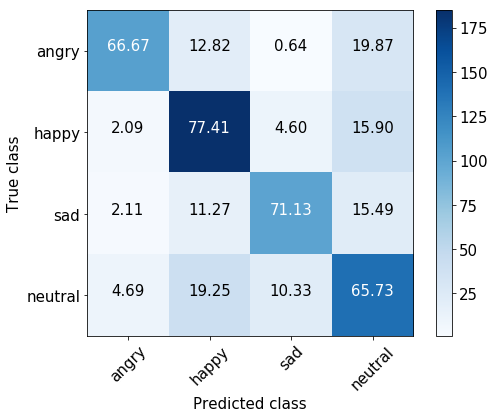}}
\caption{
Confusion matrix of each model.
}
\label{fig_confusion_appendix}
\end{figure*}
